# Supplementary material for: From Long News to Accurate Forecast: Importance-Aware Fusion and PRM-Guided Reflection for Time Series Forecasting
Source: arXiv:2606.03097 source file (2026-06-02)
Supplement: Supplementary file 1 [file appendix_standalone.tex]

% Standalone document to preview the appendix (compile with pdflatex or xelatex)
\documentclass[11pt,a4paper]{article}

\usepackage[margin=1in]{geometry}
\usepackage{booktabs}
\usepackage{graphicx}
\usepackage{multirow}
\usepackage{xcolor}
\usepackage{enumitem}
\usepackage{caption}
\usepackage{subcaption}
\usepackage{amssymb}
\usepackage{hyperref}

\title{Supplementary Appendix\\PRM-Guided News Selection and Compression}
\author{}
\date{}

\begin{document}
\maketitle
\appendix
\input{appendix_supplementary}
\end{document}
